# Supplementary material for: Well-posedness and simulation of weak solutions to the time-fractional Fokker-Planck equation with general forcing
Source: arXiv:2307.16615 source file (2023-07-31)
Supplement: Supplementary file 1 [file A_appendix.tex]

\appendix
\section{Derivation of the time-fractional Fokker--Planck equation} \label{App:Derivation}

Let $t$ denote the current time state, and let $x=x(t)$ be the space variable depending on $t$. We consider a particle being dragged through a fluid and are interested in the forces involved.
We exert on the particle an external force $F_\ext$ proportional to the gradient of the potential $U$ it encounters. Typically, it is dependent on space and time.
In addition, it is countered by the fluid's drag force $F_\drag$.
The drag or damping acts as resistance to the particle's motion, which is the outcome of the particle's attempt to shift the fluid out of the way.
A drag force requires motion, and hence it is proportional to the particle's velocity. The friction coefficient $\zeta$ is the proportionality constant that determines the damping magnitude, i.e., \begin{equation}
\label{Eq:Drag}
F_\drag=-\zeta \ddt x.
\end{equation}

Microscopically, we also recognize that the molecules of a fluid impose time-dependent random forces $F_\ran$, such as random collisions, on a molecule.
So that the specific molecular details of solute–solvent collisions can be averaged out, one considers a nanoscale solute in water (e.g., biological macromolecules) with dimensions large enough that its position is simultaneously influenced by multiple solvent molecules, but light enough that the constant interactions with the solvent leave an unbalanced force acting on the solute at any given moment.

According to Newton's second law, the acceleration of this particle is equal to the sum of these forces: 
\begin{equation} \label{Eq:Newton} m \Big(\ddt \Big)^2 x = F_\drag + F_\ext +F_\ran.
\end{equation}
%or simplified
%The drag force is present regardless of whether an external force is present, so in the absence of external forces the equation of motion governing the spontaneous fluctuations of this solute is determined from the forces due to drag and the random fluctuations:
%$$m \Big(\ddt \Big)^2 x + \partial_x U+ \zeta  \ddt  x -F_\ran =0.$$
This equation of motion is called the Langevin equation.
Moreover, since it incorporates a time-dependent random force, we  refer to it as a stochastic equation.
Incorporating a random process into a deterministic equation necessitates the employment of a statistical method to solve the problem.

We shall attempt to describe the particle's average and root-mean-squared position.
What can we say about the random force initially?
Even while there may be instant imbalances, the average perturbations from the solvent on a bigger particle will be zero at equilibrium, i.e., $\langle F_\ran \rangle=0$, notwithstanding the possibility of momentary imbalances.
It appears to imply that the drag force and the random force are independent, but in reality, they stem from the same molecular forces.
%If the molecule of interest is a protein that is exposed to the fluctuations of numerous quickly moving solvent molecules, then the averaged forces due to random fluctuations and the drag forces are connected.
The fluctuation-dissipation theorem \cite[Section 9.2]{pavliotis2014stochastic} is the general link between friction and the random force's correlation function, and in the Markovian limit it reads 
$$\langle  F_\ran(t)F_\ran(t')\rangle=2\zeta  k_B\mu_T\delta(t-t'),$$
where $\mu_T$ denotes the absolute temperature, $k_B$ the Boltzmann constant, and $\delta$ the Dirac-delta functional. Thanks to Einstein's formula, the diffusion constant reads $D=\frac{k_B\mu_T}{\zeta }$, see \cite[Example 9.8]{pavliotis2014stochastic}.

We introduce a Gaussian distributed sequence $R(t)$ of random numbers with $\langle R(t)\rangle=0$ and $\langle R(t)R(t')\rangle=\delta(t-t')$. We are in the setting of Brownian dynamics simulations and therefore, the equation of motion is diffusion-dominated, i.e., in the strong friction limit it holds $|m (\ddt)^2 x|\ll |\zeta \ddt x|$. Therefore, we can neglect inertial motion, and set the acceleration of the particle to zero. Hence, we can insert the representation of the drag force, see \Cref{Eq:Drag} into Newton's second law \Cref{Eq:Newton} to obtain an expression for the velocity of the particle
$$\ddt x=F_\ext(x(t),t)+\sqrt{2 D} R(t)$$
or in the form of a stochastic differential equation
$$\dd X_t=F_\ext(X_t,t) \dt +\sigma \dd W_t,$$
where $W_t$ is the corresponding Wiener process, and we defined $\sigma:= \sqrt{2D}$. We note that $B_t$ is a Brownian force with $B_t\dt=\sigma \dd W_t$.

%Moreover, $\zeta $ denotes the drag coefficient and the drag force is governed by the Stokes law, which in a fluid moving with velocity $u(x,t)$ reads $\zeta \big(u(x,t)-\ddt  x(t)\big)$.
%Taking the assumptions of the forces into consideration, Newton's second law reads
%$$\zeta  (\dd x(t) - u(x(t),t) \dt) = F(q(t)) \dt + \sqrt{2k_B \mu_T \zeta } \dd W(t).$$
%We divide this equation by $\zeta $ and define
%We define
%\begin{equation} \label{Def:Vectorb} X(t):=x(t), \quad b(X(t),t):=F_\ext(x(t),t), \quad ,\end{equation}
%which yields the stochastic differential equation 
%\begin{equation*} %
%\dd X(t) = b(X(t),t) \dt + \sigma \dd W(t). \end{equation*}

At this point, one can derive the typical Fokker--Planck equation,
see \cite[Section 5.3.2]{pavliotis2014stochastic}. However, we consider the subordination of the Langevin equation, i.e., %
the inverse of the subordinator becomes the operational time of the system. Physically, this means that one introduces trapping events to the motion of the particles.
The parent process $X$ is assumed to satisfy the following subordinated Langevin equation: \begin{equation} \label{Eq:Langevin} \dd X_t = F_\ext\big(X_t,U^\alpha_t\big) \dt + \sigma \dd W_t. \end{equation} 
Here, $U^\alpha_t$ is defined as a L\'evy process with nonnegative increments, see \cite[Definition 21.4, Example 21.7]{sato1999levy}, and
the inverse of $U^\alpha_t$ reads $S^\alpha_t:=\inf\{\tau:U^\alpha_\tau > t\}$. Its Laplace transform reads, see \cite[Example 24.12]{sato1999levy},  %
$$\langle  e^{-nS^\alpha_t}\rangle=E_\alpha(-nt^\alpha)=\sum_{j=0}^\infty \frac{(-n^2t^\alpha)^j}{\Gamma(j\alpha+1)},$$
where $E_\alpha$ is called the Mittag--Leffler function, see \cite{diethelm2010analysis}.
This step is essential to the derivation of the time-fractional PDE and explains why the fractional derivative appears in the mathematical model.
The Mittag-Leffler function has been used as a phenomenological physical model for exponential relaxation at short times and power law relaxation at long times; for further information, consult the book \cite{west2003physics} on the physics of fractional operators. 

We integrate the subordinated Langevin equation \cref{Eq:Langevin} on the time interval $(0,t)$, and like this, the subordinated process $Y^\alpha_t:=X_{S^\alpha_t}$ satisfies the integral equation
$$Y^\alpha_t=\int_0^t F_\ext(X_\tau,\tau) \dd S^\alpha_\tau + \sigma W_{S^\alpha_t}.$$
%where the Lebesgue--Stieltjes integral of $b$ is meant in the sense that each component of $b$ is integrated, and the result is again a vector. 
As proved in \cite[Proof of Theorem 1]{magdziarz2009stochastic}, the Fourier transform of $Y^\alpha_t$ is holomorphic in a neighborhood of zero and therefore, it is well-known that the moments uniquely determine the distribution, e.g., see \cite[Section VII.3]{feller1971introduction}. The moments are computed in \cite[Equation (11)]{sokolov2006field} and \cite[Proof of Theorem 1]{magdziarz2009stochastic}. Finally, we can conclude that the moment $\psi(t):=\langle  Y^\alpha_t \rangle$  satisfies 
\begin{equation} \label{Eq:DerivFP}
\pt \psi(x,t)= -\partial_x \left(F_\ext(x,t) \ptb \psi(x,t) \right) + D \partial_{x}^2 \ptb \psi(x,t),\end{equation}
which we call the time-fractional Fokker--Planck equation.
